# Supplementary material for: The effect of smooth parametrizations on nonconvex optimization landscapes
Source: arXiv:2207.03512 source file (2024-03-04)
Supplement: Supplementary file 1 [file appendix_desingularization_intrinsic.tex]

\section{The desingularization lift for bounded-rank matrices} \label{adpx:desingularizationlift}

\TODO{I didn't take the quotient here, to avoid a discussion about horizontal spaces etc. In any case, this is enough: once we have all the claims for the total space lift, we can get the results for the quotient lift with a couple of references to results in my book~\cite{optimOnMans}.
Currently, Exercise~{9.8} shows local minima are preserved, then Exercise~9.45 shows 1-critical points and also 2-critical points are preserved. These are in Sections 9.1 and 9.11 respectively.}

\begin{align*}
	\calM = \left\{ (X, Y) \in \Rmn \times \reals^{n \times (n-k)} : XY = 0 \textrm{ and } Y\transpose Y = I_{n-k} \right\}.
\end{align*}
\begin{align*}
	\rank(X) + \dim\ker(X) = n \textrm{ and } \dim\ker(X) \geq n-k \implies \rank(X) \leq k.
\end{align*}
\begin{align*}
	\T_{(X, Y)} \calM & = \{ (\dot X, \dot Y) \in \Rmn \times \reals^{n \times (n-k)} : \dot X Y + X\dot Y = 0 \textrm{ and } \dot Y\transpose Y + Y\transpose \dot Y = 0 \}.
\end{align*}
Equip $\Rmn \times \reals^{n \times (n-k)}$ with the usual product metric, where each of $\Rmn$ and $\reals^{n \times (n-k)}$ is equipped with the usual Euclidean inner product.
Further let $\calM$ be a Riemannian submanifold of that Euclidean space.
\begin{lemma} \label{lem:normalspacedesingularization}
	The tangent and normal spaces to $\calM$ at $(X, Y)$ are given respectively by
	\begin{align*}
		\T_{(X, Y)}\calM & = \left\{ (-X\hat B Y\transpose + \hat E, Y\Omega + \hat B) : \Omega + \Omega\transpose = 0, Y\transpose \hat B = 0 \textrm{ and } \hat E Y = 0 \right\} \textrm{ and }
		\\
		\N_{(X, Y)} \calM & = \left\{ (KY\transpose, YM + X\transpose K) : K \in \reals^{m\times(n-k)} \textrm{ and } M = M\transpose \in \reals^{(n-k)\times(n-k)} \right\}.
	\end{align*}
\end{lemma}
\begin{proof}
	Fix any $Y_\perp \in \Rnk$ such that $\begin{bmatrix} Y & Y_\perp \end{bmatrix}$ is an orthogonal matrix of size $n \times n$.
	Then, for all $\dot X \in \Rmn$ and $\dot Y \in \reals^{n \times (n-k)}$ we can write
	\begin{align*}
		\dot X & = CY\transpose + EY_\perp\transpose, & \dot Y & = Y\Omega + Y_\perp B
	\end{align*}
	with some matrices $C, E, \Omega, B$ of appropriate sizes.
	Such a pair is tangent to $\calM$ at $(X, Y)$ if and only if $C + XY_\perp B = 0$ and $\Omega + \Omega\transpose = 0$.
	This provides a more explicit description of the tangent space at $(X, Y)$:
	\begin{align}
		\T_{(X, Y)}\calM & = \left\{ (-XY_\perp BY\transpose + EY_\perp\transpose, Y\Omega + Y_\perp B) : \Omega + \Omega\transpose = 0 \textrm{ and } B, E \textrm{ free} \right\}.
		\label{eq:TXMdesingularizationparam}
	\end{align}
	(Set $\hat B = Y_\perp B$ and $\hat E = EY_\perp\transpose$ to reach the expression in the lemma statement.)
	For all $N_X \in \Rmn$ and $N_Y \in \reals^{n \times (n-k)}$ we can write
	\begin{align*}
		N_X & = KY\transpose + LY_\perp\transpose, & N_Y & = YM + Y_\perp P
	\end{align*}
	with $K, L, M, P$ of appropriate sizes.
	The pair $(N_X, N_Y)$ belongs to the normal space to $\calM$ at $(X, Y)$ if and only  if, for all $B, E$ and all skew-symmetric $\Omega$, we have
	\begin{align*}
		0 & = \inner{KY\transpose + LY_\perp\transpose}{-XY_\perp BY\transpose + EY_\perp\transpose} + \inner{YM + Y_\perp P}{Y\Omega + Y_\perp B} \\
		  & = \inner{P - Y_\perp\transpose X\transpose K}{B} + \inner{L}{E} + \inner{M}{\Omega}.
	\end{align*}
	This holds exactly if $P-Y_\perp\transpose X\transpose K = 0$, $L = 0$ and $M$ is symmetric.
	This concludes the proof since $Y_\perp P = Y_\perp^{} Y_\perp\transpose X\transpose K = (I-YY\transpose) X\transpose K = X\transpose K$.
\end{proof}
\begin{lemma} \label{lem:projdesingularization}
	The orthogonal projector from $\Rmn \times \reals^{n \times (n-k)}$ to $\T_{(X, Y)} \calM$ is given by
	\begin{align*}
		\Proj_{(X, Y)}(Z_X, Z_Y) & = \left( Z_X - KY\transpose, Z_Y - YM - X\transpose K \right)
	\end{align*}
	with $M = \symm(Y\transpose Z_Y) = \frac{1}{2}(Y\transpose Z_Y + Z_Y\transpose Y)$ and $K = (I + XX\transpose)^{-1}(Z_X Y + X Z_Y)$.
\end{lemma}
\begin{proof}
	The orthogonal projection of $(Z_X, Z_Y)$ is obtained by subtracting from it the unique normal vector such that the result is tangent.
	In other words,
	\begin{align*}
		\Proj_{(X, Y)}(Z_X, Z_Y) & = \left( Z_X - KY\transpose, Z_Y - YM - X\transpose K \right)
	\end{align*}
	with $M = M\transpose$ such that
	\begin{align*}
		(Z_X - KY\transpose)Y + X(Z_Y - YM - X\transpose K) & = 0 \textrm{ and } \\
		Y\transpose(Z_Y - YM - X\transpose K) & \textrm{ is skew-symmetric.}
	\end{align*}
	Use $XY = 0$ and $Y\transpose Y = I$ to solve these equations for $M$ and $K$.
\end{proof}
\begin{lemma}  \label{lem:LmapQmapdesingularization}
	Consider the lift $\varphi \colon \calM \to \Rmn$ defined by $\varphi(X, Y) = X$.
	Its image is the set of matrices with rank at most $k$: $\calX = \varphi(\calM) = \Rmnlk$.
	We have the following expressions and properties for the maps $\Lmap$ and $\Qmap$ of this lift:
	\begin{align*}
		\Lmap_{(X,Y)}(\dot X, \dot Y) & = \dot X, \\
		\ker \Lmap_{(X, Y)} & = \{ (\dot X, \dot Y) \colon \dot X = 0, X\dot Y = 0 \textrm{ and } \dot Y\transpose Y + Y\transpose \dot Y = 0 \}, \\
		\Qmap_{(X, Y)}(\dot X, \dot Y) & = -2(I + XX\transpose)^{-1}\dot X \dot Y Y\transpose, \\
		\Qmap_{(X, Y)}(\ker \Lmap_{(X, Y)}) & = \{ 0 \}.
	\end{align*}
\end{lemma}
\begin{proof}
	For some arbitrary $W \in \Rmn$, consider the function $\varphi_W(X, Y) = \inner{W}{\varphi(X, Y)} = \inner{W}{X}$, smooth on $\calM$.
	Recall that \TODO{eqref}
	\begin{align*}
		\innersmall{W}{\Lmap_{(X, Y)}(\dot X, \dot Y)} & = \D\varphi_W(X, Y)[\dot X, \dot Y] = \innersmall{W}{\dot X}.
	\end{align*}
	Since this holds for all $W$ we deduce by identification that
	\begin{align*}
			\Lmap_{(X, Y)}(\dot X, \dot Y) & = \dot X.
	\end{align*}
	(Of course, we could also get this result directly from differentiating $\varphi(X, Y) = X$.)
	It is then clear that the kernel of $\Lmap_{(X, Y)}$ consists of all tangent vectors with $\dot X = 0$, as claimed.
	
	From the above, we also see that the gradient of $\varphi_W$ seen as a function on all of $\Rmn \times \reals^{n \times (n-k)}$ is $(W, 0)$.
	Because $\calM$ is a Riemannian submanifold of that Euclidean space, the Riemannian gradient of $\varphi_W$ on $\calM$ is the orthogonal projection of $(W, 0)$ to the tangent spaces of $\calM$, namely: \TODO{ref book}
	\begin{align*}
		\nabla \varphi_W(X, Y) & = \Proj_{(X, Y)}(W, 0) = \left( W - KY\transpose, -X\transpose K \right) \textrm{ with } K = (I + XX\transpose)^{-1} W Y.
	\end{align*}
	Differentiate this gradient along a tangent direction $(\dot X, \dot Y)$ to find
	\begin{align*}
		\D\big( (X, Y) \mapsto \nabla \varphi_W(X, Y) \big)(X, Y)[\dot X, \dot Y] & = \left( -\dot K Y\transpose - K\dot Y\transpose, -\dot X\transpose K - X\transpose \dot K \right)
	\end{align*}
	with $\dot K = \dot H W Y + HW\dot Y$ and $H = (I + XX\transpose)^{-1}$, $\dot H = -H(\dot X X\transpose + X \dot X\transpose)H$.
	The Riemannian Hessian of $\varphi_W$ at $(X, Y)$ is obtained by orthogonal projection of the above \TODO{ref book}, that is
	\begin{align}
		\nabla^2 \varphi_W(X, Y)[\dot X, \dot Y] & = \Proj_{(X, Y)}\!\left( -\dot K Y\transpose - K\dot Y\transpose, -\dot X\transpose K - X\transpose \dot K \right).
		\label{eq:hessnablaphiWdesingularization}
	\end{align}
	To obtain an expression of $\Qmap_{(X, Y)}$, we do not need to work out this projection.
	Indeed, recall that \TODO{eqref}
	\begin{align*}
		\innersmall{W}{\Qmap_{(X, Y)}(\dot X, \dot Y)} & = \innersmall{(\dot X, \dot Y)}{\nabla^2 \varphi_W(X, Y)[\dot X, \dot Y]}_{(X, Y)}.
	\end{align*}
	Since $(\dot X, \dot Y)$ is tangent, we can also write:
	\begin{align*}
		-\innersmall{W}{\Qmap_{(X, Y)}(\dot X, \dot Y)} & = \innersmall{\dot X}{\dot K Y\transpose + K\dot Y\transpose} + \innersmall{\dot Y}{\dot X\transpose K + X\transpose \dot K} \\
			& = \innersmall{\dot K}{\dot X Y + X\dot Y} + \innersmall{K}{2\dot X \dot Y} \\
			& = \innersmall{W}{2(I+XX\transpose)^{-1} \dot X \dot Y Y\transpose}.
	\end{align*}
	(We used both $\dot X Y + X \dot Y = 0$ since $(\dot X, \dot Y)$ is tangent and the definition of $K$.)
	This holds for all $W$; therefore, by identification we deduce that
	\begin{align*}
		\Qmap_{(X, Y)}(\dot X, \dot Y) & = -2(I+XX\transpose)^{-1} \dot X \dot Y Y\transpose,
	\end{align*}
	as announced.
	Since all $(\dot X, \dot Y) \in \ker \Lmap_{(X, Y)}$ have $\dot X = 0$ in particular, it is clear that $\Qmap_{(X, Y)}(\dot X, \dot Y) = 0$ for all such vectors.
\end{proof}
\begin{lemma} \label{lem:projkerLdesing}
	The orthogonal projector from $\T_{(X, Y)}\calM$ to $\ker \Lmap_{(X, Y)}$ is given by
	\begin{align*}
		\Proj_{\ker \Lmap_{(X, Y)}}(\dot X, \dot Y) & = \left(0, \Proj_{\ker(X)} \dot Y\right),
	\end{align*}
	where $\Proj_{\ker(X)}$ orthogonally projects the columns of $\dot Y$ to the kernel of $X$ in $\Rm$.
\end{lemma}
\begin{proof}
	We must verify that the proposed projector (a) leaves the kernel of $\Lmap_{(X, Y)}$ invariant, (b) is idempotent, and (c) is self-adjoint.
	For (a), recall from Lemma~\ref{lem:LmapQmapdesingularization} that if $(\dot X, \dot Y) \in \ker \Lmap_{(X, Y)}$ then $\dot X = 0$ and $X\dot Y = 0$, that is, $\Proj_{\ker(X)} \dot Y = \dot Y$.
	For (b), notice that
	\begin{align*}
		\Proj_{\ker \Lmap_{(X, Y)}}(0, \Proj_{\ker(X)} \dot Y) = (0, \Proj_{\ker(X)}(\Proj_{\ker(X)}(\dot Y))) = (0, \Proj_{\ker(X)} \dot Y).
	\end{align*}
	Finally, for (c), we can check that for any $(\dot X, \dot Y), (\tilde X, \tilde Y) \in \T_{(X, Y)}\calM$ it holds:
	\begin{align*}
		\innersmall{(\tilde X, \tilde Y)}{\Proj_{\ker \Lmap_{(X, Y)}}(\dot X, \dot Y)} & = \innersmall{\tilde X}{0} + \innersmall{\tilde Y}{\Proj_{\ker(X)} \dot Y} \\ & = \innersmall{0}{\dot X} + \innersmall{\Proj_{\ker(X)} \tilde Y}{\dot Y} = \innersmall{\Proj_{\ker \Lmap_{(X, Y)}}(\tilde X, \tilde Y)}{(\dot X, \dot Y)}.
	\end{align*}
	This concludes the proof.
\end{proof}
\begin{theorem} \label{thm:1imp1desingularization}
	\TODO{Consider $0 < k < \min(m, n)$; we'll remove this later if ok.}
    The {\oneimpliesone} property holds at $(X, Y)$ for the desingularization lift discussed above exactly when $\rank(X) = k$.
\end{theorem}
\begin{proof}
    By Theorem~\ref{thm:1imp1charact}, we know that the {\oneimpliesone} property does not hold when $\rank(X) < k$ as then $\T_X\calX$ is not a linear space. \TODO{Eqref where we state the tangent cone to bounded rank matrices; check corner cases}
    Now assume $\rank(X) = k$.
    Then, the columns of $Y$ form an orthonormal basis for $\ker(X)$; let the columns of $Y_\perp$ form an orthonormal basis for the orthogonal complement of $\ker(X)$, that is, for $\im(X\transpose)$.
    Likewise, let $U_\perp \in \Rmk$ have columns forming an orthonormal basis for $\im(X)$ and let $U \in \reals^{m \times (m-k)}$ complete that to an orthonormal basis for $\Rm$.
    Following Lemma~\ref{lem:normalspacedesingularization}, every $\dot X$ in a tangent pair $(\dot X, \dot Y)$ is of the form $\dot X = -XY_\perp BY\transpose + EY_\perp\transpose$ for some $B, E$ of appropriate sizes.
    Further split $E$ as $E = UU\transpose E + U_\perp^{} U_\perp\transpose E = UE_0 + U_\perp E_1$ with the obvious definitions for $E_0, E_1$.
    It follows that
    \begin{align*}
        \Lmap_{(X, Y)}(\dot X, \dot Y) & = \dot X = \begin{bmatrix} U_\perp & U \end{bmatrix} \begin{bmatrix} E_1 & -U_\perp\transpose X Y_\perp^{} B  \\ E_0 & -U\transpose X Y_\perp B \end{bmatrix} \begin{bmatrix} Y_\perp\transpose \\ Y\transpose \end{bmatrix}.
    \end{align*}
    Since $U_\perp\transpose X Y_\perp^{} \in \Rkk$ is invertible and $U\transpose X = 0$, it follows from \TODO{eqref tangent cone bounded rank} that $\im \Lmap_{(X,Y)} = \T_X\Rmnlk$: conclude with Theorem~\ref{thm:1imp1charact}.
\end{proof}
\begin{theorem} \label{thm:2imp1desingularization}
	\TODO{Consider $0 < k < \min(m, n)$; we'll remove this later if ok.}
	The {\twoimpliesone} property holds for the desingularization lift discussed above, yet none of the sufficient conditions from Theorem~\ref{thm:2imp1sufficient} hold at points $(X, Y)$ such that $\rank(X) < k$.
\end{theorem}
\begin{proof}
	We first argue that the sufficient conditions in Theorem~\ref{thm:2imp1sufficient} do not hold at points $(X, Y)$ such that $\rank(X) < k$.
	Indeed, $\Qmap_{(X, Y)}(\ker \Lmap_{(X, Y)}) = \{ 0 \}$ (by Lemma~\ref{lem:LmapQmapdesingularization}) implies that $(\Qmap_{(X, Y)}(\ker \Lmap_{(X, Y)}))^* = \Rmn$.
	Thus, the tightest sufficient condition would require $(\im \Lmap_{(X, Y)})^\perp \subseteq (\T_X\calX)^*$.
	Yet we always have the reverse inclusion by Lemma~\ref{lem:TyMandTxX}.
	As a result, the sufficient condition would require that we have $(\im \Lmap_{(X, Y)})^\perp = (\T_X\calX)^*$.
	We know from the proof of Theorem~\ref{thm:1Pimp1Q} that this is equivalent to having $\im \Lmap_{(X, Y)} = \T_X \calX$.
	This is impossible when $\rank(X) < k$ as then the left-hand side is a linear subspace yet the right-hand side is not. \TODO{Check last claim for corner cases.}
	
	Notwithstanding, the {\twoimpliesone} property \emph{does} hold over all of $\calM$.
	Owing to Theorem~\ref{thm:1imp1desingularization}, it only remains to show this for $(X, Y) \in \calM$ such that $\rank(X) < k$: we assume this below.
	
	To see that the {\twoimpliesone} property holds at $(X, Y)$, we call upon our characterization in Theorem~\ref{thm:2imp1charact}.
	We must show that $(\im \Lmap_{(X, Y)})^\perp \cap Z_{(X, Y)} \subseteq (\T_X\calX)^*$, where $Z_{(X, Y)}$ is as defined in~\eqref{eq:setZ}.
	This holds a fortiori if $Z_{(X, Y)} \subseteq \im\Lmap_{(X, Y)}$, as then $(\im \Lmap_{(X, Y)})^\perp \cap Z_{(X, Y)} = \{0\}$.
	Momentarily, we will argue that
	\begin{align}
		Z_{(X, Y)} & = \{ W \in \Rmnlk : (W, Y) \in \calM \} = \{W \in \Rmn : WY = 0\}.
		\label{eq:Zfordesingularization}
	\end{align}
	Assuming this is true for now, consider $(\dot X, \dot Y) = (W, 0)$ with $W \in Z_{(X, Y)}$.
	This is indeed a tangent vector since $\dot X Y + X\dot Y = WY = 0$ and $\dot Y\transpose Y + Y\transpose \dot Y = 0$.
	Moreover, $\Lmap_{(X, Y)}(\dot X, \dot Y) = W$.
	Therefore, $W \in \im\Lmap_{(X, Y)}$, that is, $Z_{(X, Y)} \subseteq \im\Lmap_{(X, Y)}$.
	
	It remains to verify eq.~\eqref{eq:Zfordesingularization}.
	We do so in two steps.
	Given an arbitrary $W \in \Rmn$, we first show that
	\begin{align}
		\im\!\left( \Proj_{\ker \Lmap_{(X, Y)}} \circ \nabla^2 \varphi_W(X, Y) \circ \Proj_{\ker \Lmap_{(X, Y)}} \right) = \{0\},
		\label{eq:desingularizationimProjnablaA}
	\end{align}
	then we show that
	\begin{align}
		\im\!\left( \Proj_{\ker \Lmap_{(X, Y)}} \circ \nabla^2 \varphi_W(X, Y) \right) = \{0\} && \iff && WY = 0,
		\label{eq:desingularizationimProjnablaB}
	\end{align}
	where $\varphi_W(X, Y) = \inner{W}{X}$ is a function on $\calM$ and $\nabla^2 \varphi_W$ is its Riemannian Hessian, as in the proof of Lemma~\ref{lem:LmapQmapdesingularization}.
%	\TODO{To be continued; for $k \geq 1$ it's easy to show that $\nabla^2 \varphi_W = 0$ iff $WY = 0$, but that's not quite what we need; the first claim with the two projectors is similarly easy; but the one with a single projector I'm afraid we'll need to develop full expressions for the Hessian... Actually, if $WY = 0$, then we are good; if $WY \neq 0$, then we know that the Hessian is nonzero, and we need to exhibit a tangent vector whose image through the Hessian is not orthogonal to the kernel of $\Lmap_{(X, Y)}$: that's enough to show the image is not trivial.}

	Continuing from~\eqref{eq:hessnablaphiWdesingularization}, we proceed to compute the Hessian of $\varphi_W$:
	\begin{align*}
		\nabla^2 \varphi_W(X, Y)[\dot X, \dot Y] & = \left( Z_X - \tilde K Y\transpose , Z_Y - Y\tilde M - X\transpose \tilde K \right)
	\end{align*}
	with \TODO{early on, define $\symm$ and $\skeww$ operators}
	\TODO{We could skip a few steps here, by introducing the general formula for $\Proj_{\ker \Lmap_{(X, Y)}} \circ \Proj_{(X, Y)}$.}
	\begin{align*}
		H & = (I + XX\transpose)^{-1}, & \dot H & = -H(\dot X X\transpose + X \dot X\transpose)H, \\
		K & = H W Y, & \dot K & = \dot H W Y + HW\dot Y, \\
		Z_X & = -\dot K Y\transpose - K\dot Y\transpose, & Z_Y & = -\dot X\transpose K - X\transpose \dot K, \\
		\tilde M & = \symm(Y\transpose Z_Y), & \tilde K & = H(Z_X Y + XZ_Y).
	\end{align*}
	Combining with Lemma~\ref{lem:projkerLdesing}, the projection of the Hessian to the kernel of $\Lmap$ is simply:
	\begin{align*}
		\Proj_{\ker \Lmap_{(X, Y)}}\!\left(\nabla^2 \varphi_W(X, Y)[\dot X, \dot Y]\right) & = \left( 0 , \Proj_{\ker(X)}(Z_Y) - Y\tilde M \right) \\
			& = \left( 0, -\Proj_{\ker(X)}(\dot X\transpose K) + Y\symm(Y\transpose \dot X\transpose K) \right).
	\end{align*}
	Whenever $(\dot X, \dot Y)$ is in $\ker \Lmap_{(X, Y)}$ (which implies $\dot X = 0$ in particular), the above is zero: this establishes~\eqref{eq:desingularizationimProjnablaA}.
	Moreover, if $WY = 0$ then $K = 0$ and it similarly follows that the above is zero: this establishes one direction of~\eqref{eq:desingularizationimProjnablaB}.
	To verify the other direction, assume $W$ is such that the above is zero for all $(\dot X, \dot Y) \in \T_{(X, Y)} \calM$: we must show that this implies $WY = 0$.
	Equivalently, we must show that this implies $K = 0$ (since $H$ is always invertible).
	Following Lemma~\ref{lem:normalspacedesingularization}, every $\dot X$ takes the form $\dot X = -X\hat B Y\transpose + \hat E$ with $Y\transpose \hat B = 0$ and $\hat EY = 0$, so
	\begin{align*}
		\dot X\transpose K & = -Y\hat B\transpose X\transpose K + \hat E\transpose K, & Y\transpose \dot X\transpose K & = -\hat B\transpose X\transpose K.
	\end{align*}
	Therefore,
	\begin{align*}
		-\Proj_{\ker(X)}(\dot X\transpose K) + Y\symm(Y\transpose \dot X\transpose K) & = Y\hat B\transpose X\transpose K - \Proj_{\ker(X)}(\hat E\transpose K) - Y\symm(\hat B\transpose X\transpose K) \\
			 & = Y\skeww(\hat B\transpose X\transpose K) - \Proj_{\ker(X)}(\hat E\transpose K).
	\end{align*}
%	For contradiction, assume $K \neq 0$.
%	We consider two cases.
%	\textbf{In the first case}, $\rank(X) = k$; equivalently, % to see the equivalence, just write rank(X) + null(X) = n: this doesn't depend on any relation between m and n.
%	$\ker(X) = \im(Y)$ and $\Proj_{\ker(X)} = YY\transpose$.
%	Since we also have $\hat E Y = 0$, it follows that $Y\skeww(\hat B\transpose X\transpose K) = 0$, that is, $\hat B\transpose X\transpose K$ is symmetric for all $\hat B$ such that $Y\transpose \hat B = 0$.
%	\TODO{Let $\hat B = X\transpose G$ for some arbitrary $G \in \reals^{m \times (n-k)}$---this is the same size as $K$; it holds indeed that $Y\transpose \hat B = 0$. For contradiction, assume $K \neq 0$. To conclude, we must construct $G$ such that $G\transpose XX\transpose K$ is not symmetric. First, we need to ensure $X\transpose K$ is nonzero, or handle that case separately... Bottomless annoyance. Either there's still a mistake somewhere, or what we can show is that the image of Proj Hess is trivial iff $X\transpose K = 0$ (instead of $K = 0$, that is $WY = 0$)---would that be enough for our final goal?}
%	\textbf{In the second case}, $\rank(X) < k$.
    Recall that we assume $\rank(X) < k$.
	Therefore, there exists a unit vector $z \in \Rn$ such that $Xz = 0$ yet $Y\transpose z = 0$.
	For an arbitrary vector $u \in \Rm$, let $\hat E = uz\transpose$ and $\hat B = 0$ (notice that $\hat E Y = 0$).
	It follows that
	\begin{align*}
		0 & = Y\skeww(\hat B\transpose X\transpose K) - \Proj_{\ker(X)}(\hat E\transpose K) = zu\transpose K
	\end{align*}
	for all $u \in \Rm$, therefore implying that $K = 0$.
	
	\TODO{As a concluding remark, note that $Z_{(X, Y)}$ may be different from $\{ W : WY = 0 \}$ when $\rank(X) = k$, as then it is easy to see that $Z_{(X, Y)}$ contains $\{ W : X\transpose H W Y = 0 \} = \{ W : X\transpose W Y = 0 \}$ which, in general, may be strictly larger than $\{ W : WY = 0 \}$. Also, it is not included in $\im\Lmap_{(X, Y)}$ so the above proof doesn't work.---we could include this, but if we do, we should vet it; leaving this in red for now.}
\end{proof}
